# Supplementary material for: libmpk: Software Abstraction for Intel Memory Protection Keys
Source: arXiv:1811.07276 source file (2018-11-18)
Supplement: Supplementary file 1 [file appendix.tex]

\clearpage
\appendix

\section{Sample Code}

\begin{figure}[h]
  \input{code/pkey-wrap.c}
  \coderule
%   \input{code/pkey-libc-func.c}
%   \coderule
  \caption{Wrapper functions for \rdpkru and \wrpkru from glibc 2.27.}
  \label{c:pkru}
\end{figure}

\begin{figure}[h]
 \input{code/exec-only.c}
 \coderule
  \caption{An example code for making execute-only pages with
    MPK-enabled \mprotect (error handlings are omitted for brevity).}
 \label{c:exec-only}
\end{figure}

%\begin{figure}[t]
%  \input{code/openssl.ori.c}
%  \caption{openssl original code in rsa/rsa\_pmeth.c}
%  \label{c:sslori}
%\end{figure}
\begin{figure}[h]
  \input{code/openssl.mpk.c}
  \coderule
  \caption{decrypt function with private key in rsa/rsa\_pmeth.c}
  \label{c:sslmpk}
\end{figure}

\begin{figure}[h]
  \input{code/mc.c}
  \coderule
  \caption{do_store_item function in memcached.c}
  \label{c:mcmpk}
\end{figure}

\begin{figure}[h]
  \input{code/microbench.js}
  \coderule
	\caption{The microbenchmark for evaluating the cache performance of
	applying \emph{one key per page} approach in JIT compilation to ensure
	W$\oplus$X. During the execution of N.js, ChakraCore compiles and further
	optimizes N hot functions within N + 1 executable pages on-the-fly.}
  \label{c:microbench-js}
\end{figure}
